# Supplementary material for: Conditional Generative Refinement Adversarial Networks for Unbalanced Medical Image Semantic Segmentation
Source: arXiv:1810.03871 source file (2018-10-09)
Supplement: Supplementary file 1 [file appendix.tex]

\section{supplementary material} \label{appendix}

%\subsection{Networks Architecture}

\begin{figure*}
  \centering
  \subfloat[]{\includegraphics[width=0.75\textwidth]{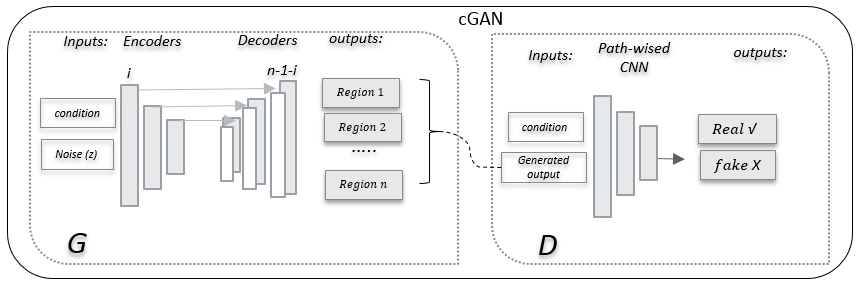}\label{fig_a}}
  \hfill
  \subfloat[]{\includegraphics[width=0.72\textwidth]{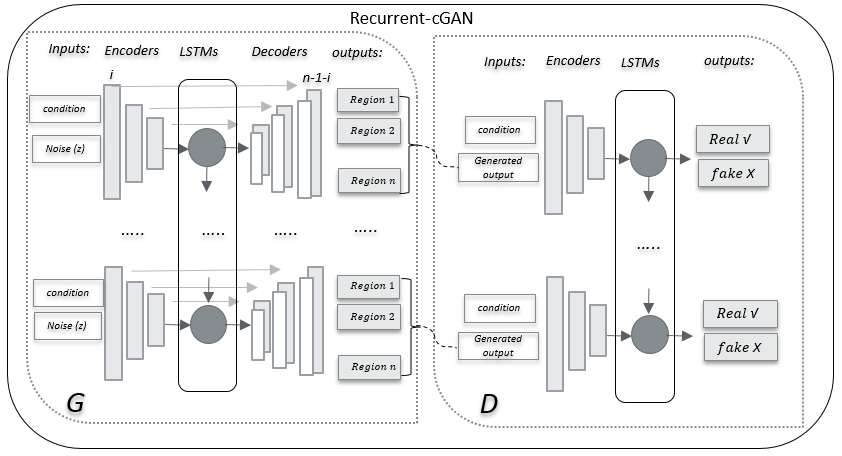}\label{fig_b}}
  \hfill
  \subfloat[]{\includegraphics[width=0.75\textwidth]{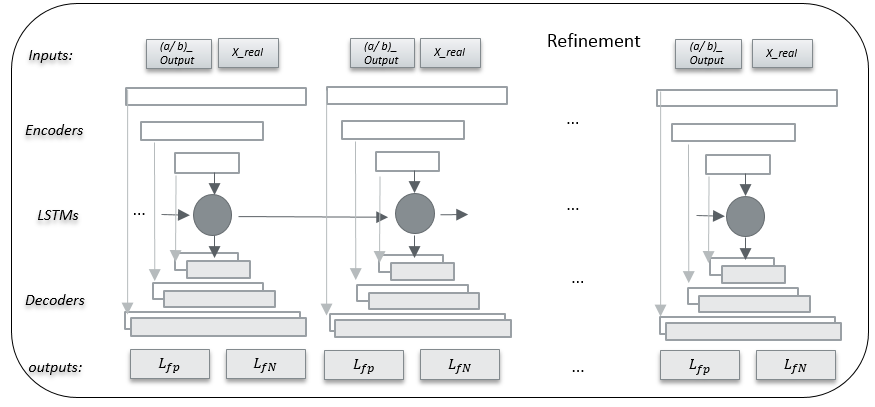}\label{fig_c}}
  \caption{The architecture of our proposed network in the two stages of semantic segmentation and segmentation label refinement for mitigating imbalanced data issue.
We designed two different architectures for the first stage a conditional GAN and a recurrent conditional GAN which are respectively shown in (a) and (b). Our cGAN architecture (a) comprises a generator and a discriminator network.
The generator is UNet architecture with a skip connection between the convolutions where it learns the segmentation label's map.
The discriminator network is a fully convolutional neural network (FCN) that discriminates segmentation maps coming from ground truth or from the generator network.
Similarly, the recurrent-cGAN architecture (b) has a generator and a discriminator network, where both have been substituted by recurrent neural networks.
In the second stage, refinement network (c) is trained on the error mask predicted by one of the architectures (a) or (b) from the first stage.
The final semantic segmentation masks computed by eliminating false positives and adding false negatives masks to the first stage output.}
\end{figure*}

%\subsection{Data Preparation}

\begin{figure*} [!t]
\includegraphics[width=0.95\textwidth]{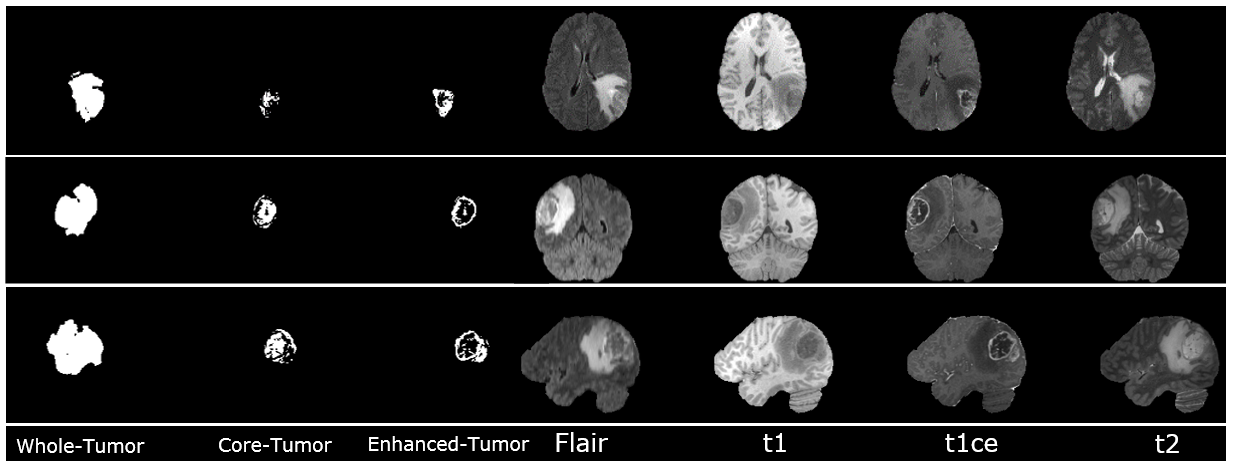}
\centering
\caption{ The brain MR image, (Brats17-CBICA-AAP-1) from BraTS2017 after pre-processing, with each patient having five modalities. We extracted the segmentation mask from the GT file for each sub-region of tumor.}
\label{fig_preprocess_brain}
\end{figure*}

\begin{figure*} [!t]
\includegraphics[width=0.95\textwidth]{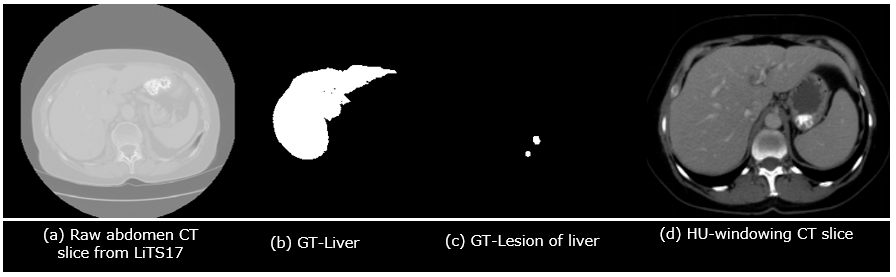}
\centering
\caption{The CT image, from LiTS2017 before and after pre-processing. We extracted two segmentation masks from the ground truth file annotated by medical expert for liver and lesion(s) respectively.}
\label{fig_preprocess_liver}
\end{figure*}

\begin{figure*} [!t]
\includegraphics[width=0.95\textwidth]{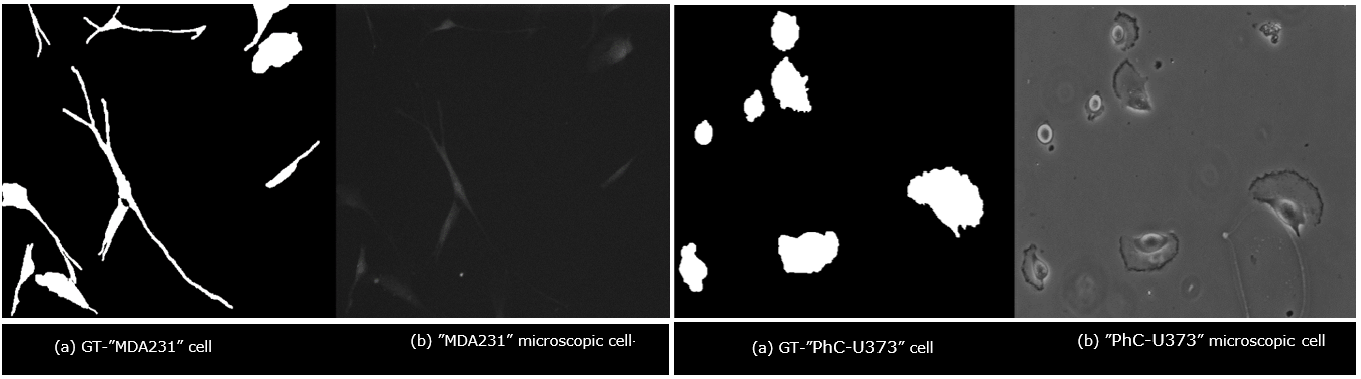}
\centering
\caption{ The microscopic cell images collected from cell segmentation challenge 2015. The network is trained on two datasets the MDA231 images (left-b) with the binary mask (left-a), and the PhC-HeLa image (right-b) with the ground truth mask annotated by the medical expert (right-a).}
\label{fig_preprocess_cell}
\end{figure*}

%\subsection{Qualitative Results}

\begin{figure*}[!htbp]
\includegraphics[width=0.95\textwidth]{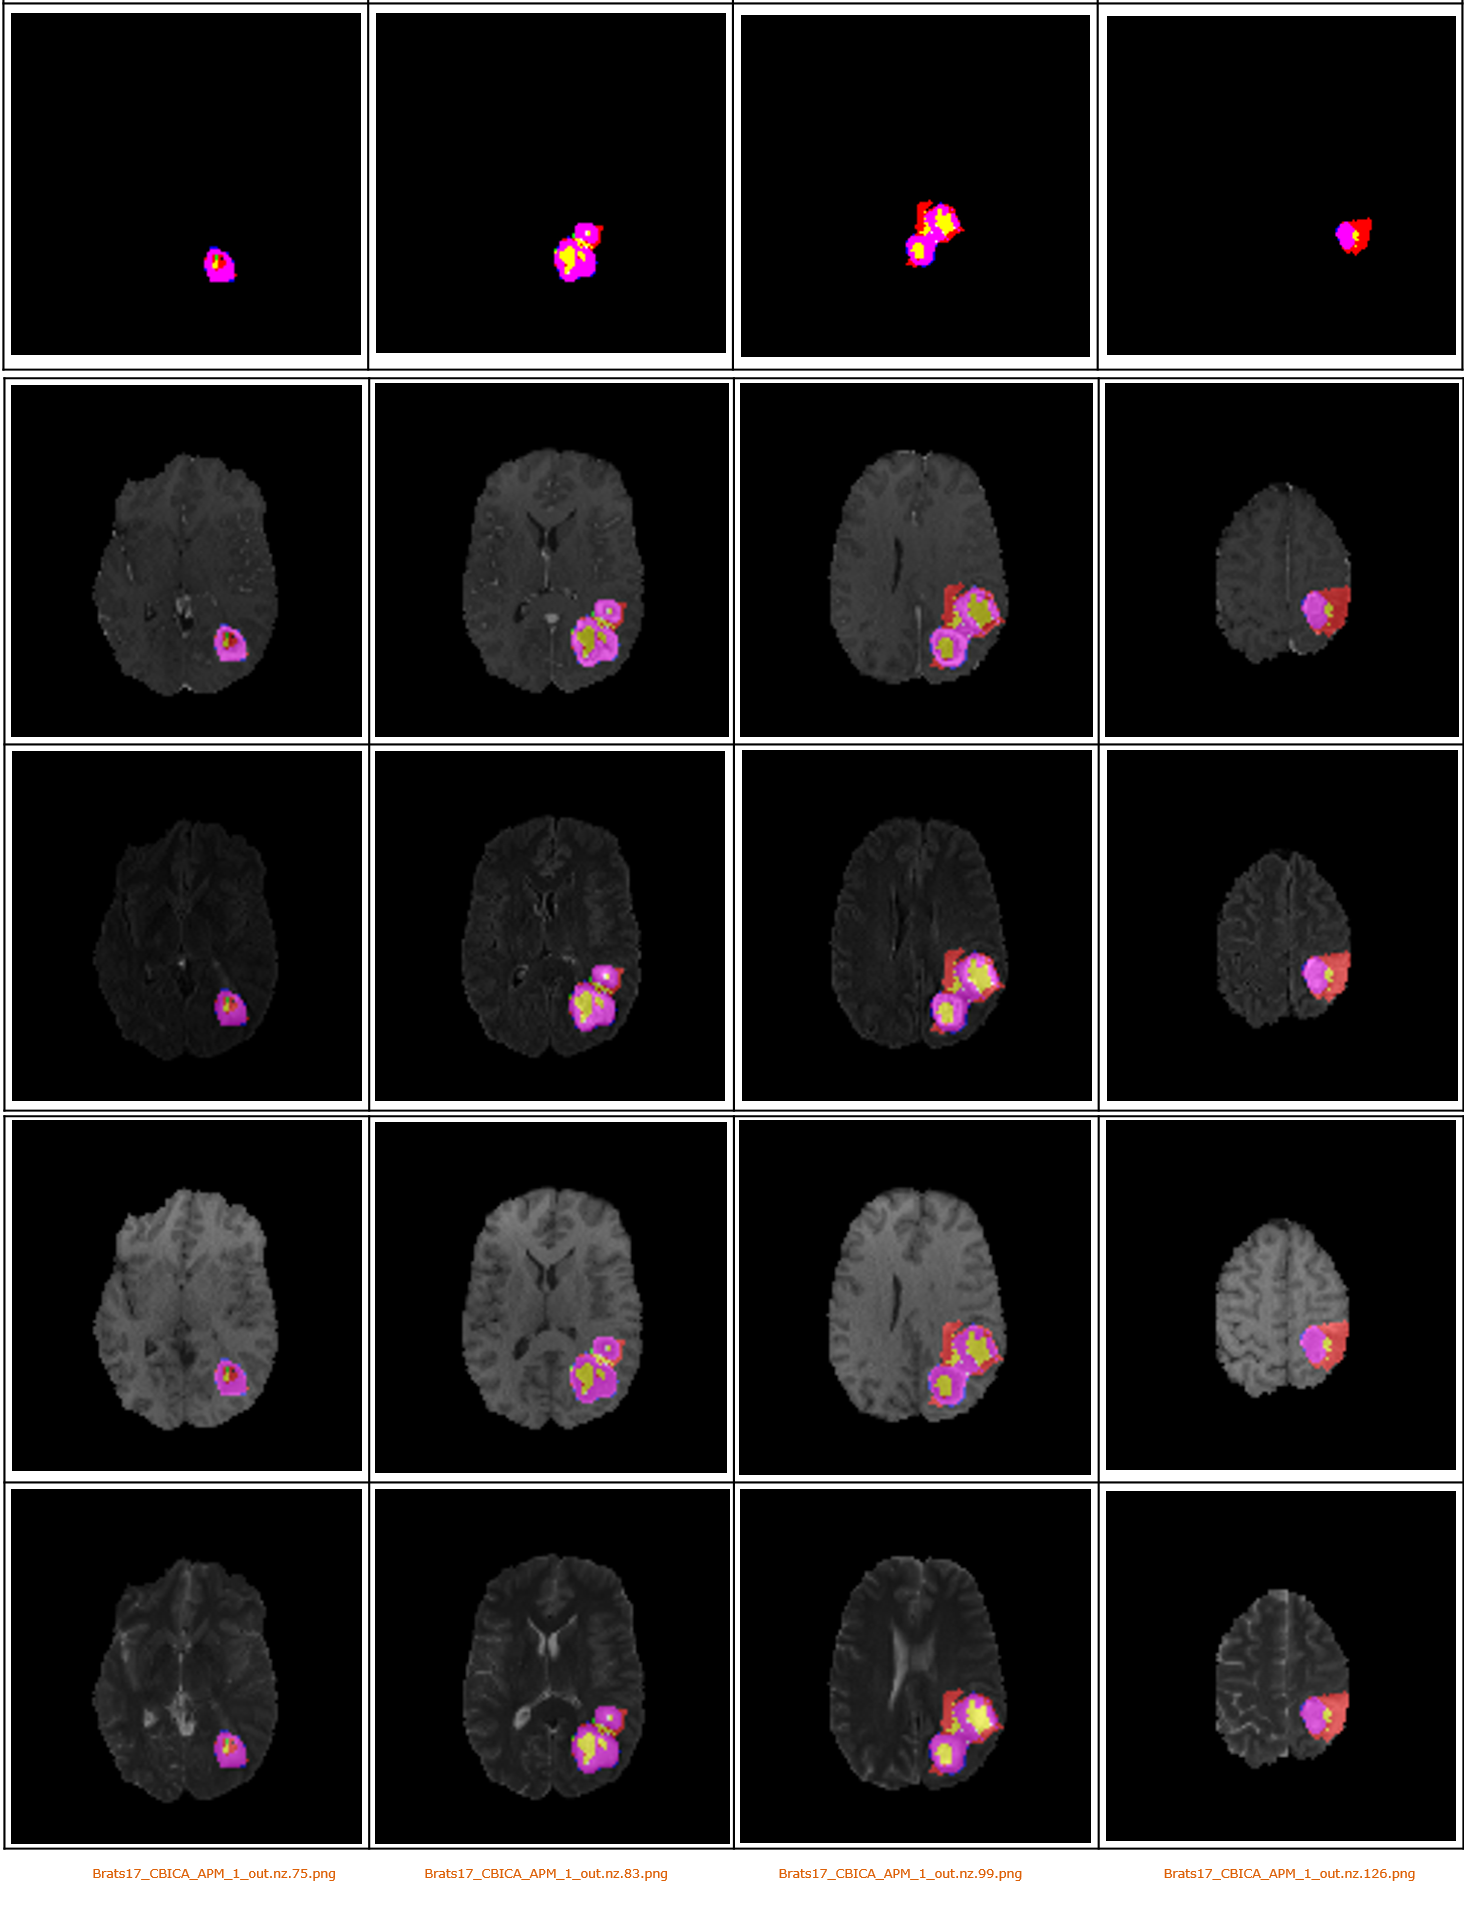}
\centering
\caption{Example results produced by our method from Brats17-CBICA-APM at a test time. The first row shows the final output with couple tumours, and other rows show the overlaid predicted semantic masks on the MRI modalities. The red color codes the whole tumour region (WT), likewise pink and yellow represent enhanced tumour (ET) and tumorous core (CT) respectively.}
\label{fig_rnngan}
\end{figure*}

\begin{figure*}[!htbp]
\includegraphics[width=0.99\textwidth]{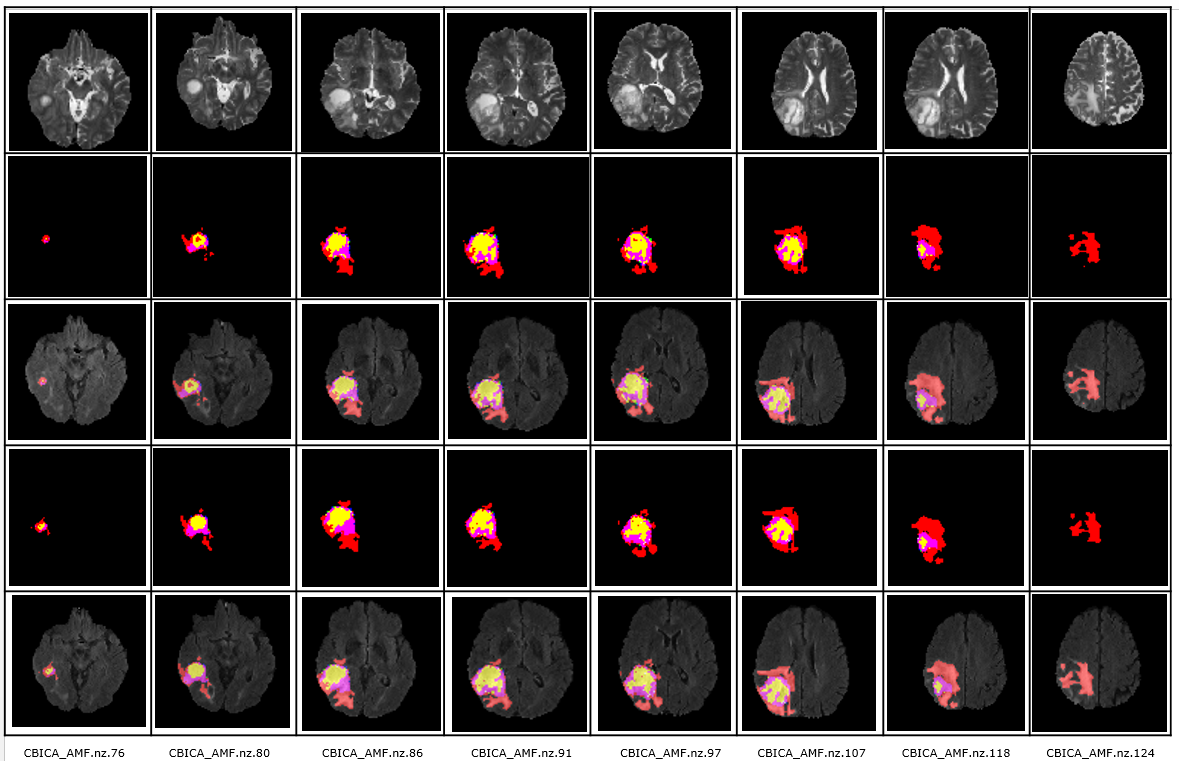}
\centering
\caption{Visual results from our model on axial views of CBICA-AMF.nz.76-124 from the validation set. The first row shows Flair modality, while the second and fourth row show the output results respectively from cGAN and refinement architecture. The third row shows the semantic segmentation masks from cGAN overlaid Flair modalities where the fifth row shows outputs after refinement network. The red color codes the whole tumour (WT) region, while pink and yellow represent the enhanced tumour (ET) and the tumorous core (TC) respectively.}
\label{fig_brain_ex1}
\end{figure*}

\begin{figure*} [!t]
\includegraphics[width=0.99\textwidth]{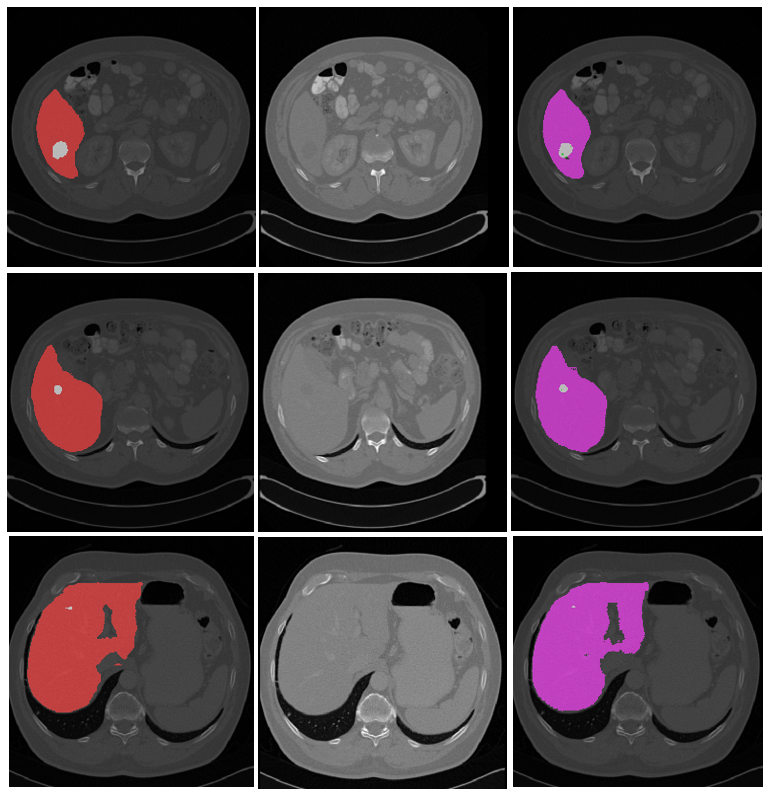}
\centering
\caption{Axial view of segmentation results from our proposed architecture. The left column shows the ground truth file annotated by a medical expert, while the middle column and the right column show the input slides and  predicted results by ours respectively. The red color depicts the ground truth region and pink color shows the predicted output by us. }
\label{fig_livrescolor}
\end{figure*}

\begin{figure*}[!t]
  \centering
  \subfloat[]{\includegraphics[width=0.48\textwidth]{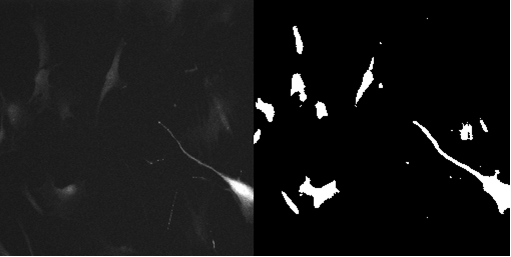}\label{figa}}
  \hfill
  \subfloat[]{\includegraphics[width=0.48\textwidth]{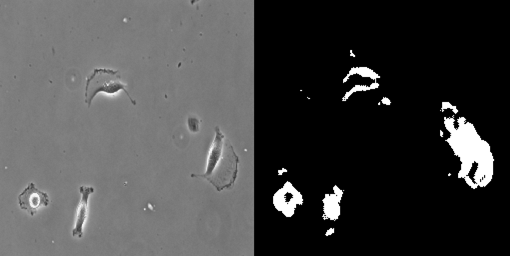}\label{figb}}
  \caption{Microscopic cell segmentation results obtained by cGAN (a,b) when the cGAN model trained  with additional Gaussian noise as input.}
\label{fig_cellnoise}
\end{figure*}

\begin{figure*}[!t]
  \centering
  \subfloat[]{\includegraphics[width=0.48\textwidth]{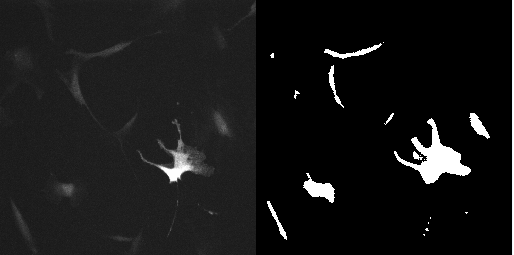}\label{figaa}}
  \hfill
  \subfloat[]{\includegraphics[width=0.48\textwidth]{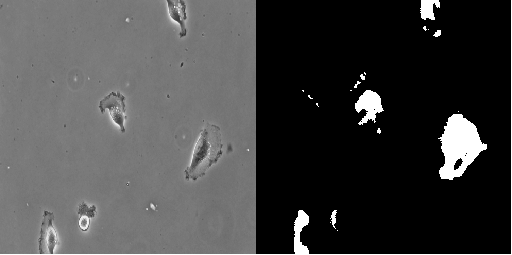}\label{figbb}}
  \caption{Microscopic cell segmentation results obtained by cGAN (a,b) without patient-wise mini-batch normalization.}
\label{fig_cellschaffel}
\end{figure*}
